# Supplementary material for: SDGOCC: Semantic and Depth-Guided Bird's-Eye View Transformation for 3D Multimodal Occupancy Prediction
Source: arXiv:2507.17083 source file (2025-07-22)
Supplement: Supplementary file 1 [file X_suppl.tex]

\clearpage
\setcounter{page}{1}
\maketitlesupplementary
\appendix
\section{Point-to-Pixel Correspondence}
\label{sec:img_point}
We can obtain the index between points and image pixels using the given extrinsic ${T_{\scriptscriptstyle \mathit{ex}}}$ matrix between sensors and the camera's intrinsic ${K}$ matrix. Each point includes 3D coordinates (${x}, {y}, {z}$) and the obtained 2D projection pixel coordinate $^{C}{p}_{i}=\left[\begin{array}{ll}u_{i} & v_{i}\end{array}\right] \in \mathbb{R}^{{H_C} \times{W_C}}$. To apply the coordinate transformation, we add a fourth column to turn it into a 4D vector, making the equation homogeneous. The projection process is described as follows:
\begin{equation}
\begin{aligned}
{{Z}_{i}} \: ^{C}{p}_{i}& ={{K}} {T_{\scriptscriptstyle \mathit{ex}}} \: {^{L}{p}}_{i}  \\
& ={{K}} [{R} \mid {t}] \left[\begin{array}{llll} x_{i} &y_{i} &z_{i} &1 
\end{array}\right]^{T},
\end{aligned}
\end{equation}
\begin{equation}
{T_{\scriptscriptstyle \mathit{ex}}}=\left[\begin{array}{cc}
{R} & {t} \\
0 & 1
\end{array}\right],
\end{equation}
where $^{L} {p}_{i}$ and $^{C}{p}_{i}$ are the corresponding 3D point coordinates and image pixel coordinates, and ${R}$ and ${t}$ represent the rotation matrix and the translation vector in the transformation matrix ${T_{\scriptscriptstyle \mathit{ex}}}$, ${Z}_{i}$ is the depth of the 3D point.
\section{Further Implementation Details}
\label{sec:further_implement}
In this section, we further elaborate on the implementation details of our SDG-OCC.

\textbf{Evaluation Metrics.}
To evaluate the performance of our method, we use the Mean Intersection over Union (mIoU) over all classes for evaluation, which quantifies the overlap between actual and predicted values relative to their combined set. It is calculated by
\begin{equation}
\mathrm{mIoU}=\frac{1}{N} \sum_{c=1}^{N} \operatorname{IoU}_{c}=\frac{1}{N} \sum_{c=1}^{N} \frac{T P_{c}}{T P_{c}+F P_{c}+F N_{c}},
\end{equation}
\noindent where $T P_{c}, F N_{c}, F P_{c}$ denote true positives, false negatives, and false positives, respectively. After averaging the IoU values per class, the primary evaluation metric for semantic segmentation, mIoU, is derived. 

\textbf{Training Details.}
The image size is adjusted to 256×704 with normalization, padding and random flipping for image augmentation. To enhance performance, an exponential moving average (EMA) hook is adopted. Test-time augmentation techniques are not employed for BEV augmentation.

\textbf{Loss Function.} During training, we use a total of five different loss functions:
\begin{equation}
\mathcal{L} = \begin{array}{l}
\lambda_{{\rm depth}}\mathcal{L_{\rm depth}} + \lambda_{{\rm seg}}\mathcal{L_{\rm seg}} + \lambda_{{\rm pts}}\mathcal{L_{\rm pts}} \\
+ \lambda_{{\rm mask\text{-}occ}}\mathcal{L_{\rm mask\text{-}occ}}+\lambda_{{\rm kl}}\mathcal{L_{\rm distill}}
\end{array},
\end{equation}
where $\mathcal{L_{\rm depth}}$ and $\mathcal{L_{\rm seg}}$ represent the losses for depth estimation and image semantic segmentation in the view transformation, both using cross-entropy loss. $\mathcal{L_{\rm pts}}$ denotes the voxel supervision loss based on the target scale in LiDAR segmentation, integrating both Lovasz loss and cross-entropy loss. $\mathcal{L_{\rm mask\text{-}occ}}$ is the loss between the predicted occupancy grid and the ground truth (GT), employing masked cross-entropy loss. $\mathcal{L_{\rm distill}}$ is the loss function for knowledge distillation, representing the weight ratio of unidirectional knowledge transfer from multimodal to unimodal representations, where $\alpha=\beta$=1.0. And we set the hyper-parameters to $\lambda_{{\rm depth}}=0.05$ and $\lambda_{{\rm seg}}=0.5$ for the depth and segmentation losses, respectively, and additionally include weights $\lambda_{{\rm pts}}$=$\lambda_{{\rm mask\text{-}occ}}$=$\lambda_{{\rm kl}}$=1.0 to balance their contributions in the overall loss function.

\begin{table}[t]
\centering
% on overall model performance: fusion after the BEV encoder and fusion before the BEV encoder.}
\resizebox{1.0\columnwidth}{!}{%
\begin{tabular}{c|c|c|cc}
\hline
 Fusion Method &IoU(\%)  & mIoU(\%) &FLOPs(G)&Params(M)\\
\hline
\text{SDG-FB}& 95.26 & 51.32& 1159&92.1\\
\text{SDG-FA} & 95.35  & 51.66&1162&92.9 \\
\text{SDG-KL} & 95.26  & 50.16&1067&57.9 \\
 \hline
\end{tabular}
}
\caption{The ablation study on the fusion strategies.SDG-FB represents fusion after the BEV encoder, SDG-FA represents fusion before the BEV encoder,SDG-KL represents fusion and distillation. }
\label{tab:5}
\vspace{-12pt}
\end{table}
\begin{table}[t]
\centering
% on overall model performance: fusion after the BEV encoder and fusion before the BEV encoder.}
\resizebox{1.0\columnwidth}{!}{%
\begin{tabular}{c|c|c|cc|c}
\hline
 Method &IoU(\%)  & mIoU(\%) &FLOPs(G)&Params(M)&Time(ms)\\
\hline
\text{img$^\dagger$}& 94.62 & 48.51&1067&57.9&83\\
\text{img+lidar} & 95.35 & 51.66&1162&92.9& 133\\
\text{img$^\dagger$+lidar} & 95.48 & 51.71&2251&100.48& 217 \\
 \hline
\end{tabular}
}
\caption{The ablation study on the temporal fusion. $^\dagger$ represents the temporal fusion module for multi-frame images. }
\label{tab:6}
\vspace{-12pt}
\end{table}
\section{Further Experiments}
In this section, we provide more experiments of our proposed method.

\textbf{Feature Fusion Strategies.} The feature fusion strategies of the feature fusion has a significant impact on the final performance. We conducte experiments on the image BEV features obtained from the initial view transformation and those processed by the BEV encoder. According to the results in Tab. \ref{tab:5}, applying the encoder before fusion and distillation yields better performance.

\textbf{Effectiveness of Temporal Fusion.} Temporal augmentation is a crucial technique for enhancing 3D perception performance. While it introduces multi-frame information, it causes only a small increase in memory overhead yet brings substantial performance improvements. To validate the effectiveness of temporal fusion, we conducte experiments using common temporal fusion methods from BevStereo, with results shown in Tab. \ref{tab:6}. Integrating temporal information into camera-only models yields a noticeable performance improvement with minimal computational overhead and a small compromise in processing speed. However, when multimodal data is further integrated with temporal information, the improvement becomes negligible, indicating a potential intrinsic coupling between the temporal dynamics of multi-frame image sequences and LiDAR information.

\textbf{ Sensitivity to intrinsic and extrinsic.} LSS methods are sensitive to both intrinsic and extrinsic factors due to the unidirectional mapping between image pixels and 3D points. Any misalignment in the intrinsic parameters of the camera or the extrinsic parameters of the 3D scene can lead to significant errors. In contrast, our approach leverages co-points from LiDAR as priors and employs bidirectional projection between 3D points and image pixels. The perturbations in the transformation matrix have minimal impact on the bidirectional projection process, resulting in a more stable and robust mapping. Random perturbations, including translations and rotations (see Tab. \ref{tab:r1}), demonstrate that our method maintains minimal performance degradation, highlighting its robustness.
\begin{table}[t]
\centering
\resizebox{1.0\columnwidth}{!}{%
\begin{tabular}{cc|c|c}
\hline
translations (m) & rotations ($^\circ$) & IoU$\uparrow$  & mIoU$\uparrow$ \\
\hline
0.1 & 1 & -1.4\%  & -0.12\% \\
\hline
\end{tabular}
}
 % \vspace{-4pt}  % Reduce space below the table
\caption{Random perturbation on the matrix}
 \vspace{-4pt}  % Reduce space below the table
\label{tab:r1}
\end{table}

\textbf{Ablation Study on the Fusion-Distillation Module}. We conducted ablation experiments on the baseline, separately for the performance-based fusion method and the speed-based distillation method. The results are shown in Tab. \ref{tab:r3},  where it can be observed that the fusion-based method performs slightly better than the fusion-distillation method.
\begin{table}[t]
\centering
\scriptsize
\setlength{\tabcolsep}{20pt} % Adjust column spacing to increase table width
\resizebox{1.0\columnwidth}{!}{%
\begin{tabular}{c|c|c}
\hline
method & IoU  & mIoU \\
\hline
Baseline+FOAD & 94.49 \% & 43.51\% \\
Baseline+Fusion & 94.74\%  & 44.92\% \\
\hline
\end{tabular}
}
 % \vspace{-4pt}  % Reduce space below the table
\caption{Ablation experiment on the neighborhood attention}
\vspace{-12pt}  % Reduce space below the table
\label{tab:r3}
\end{table}

\section{Visualization}
\label{sec:vis}
In this section, we provide more visualization results of our proposed method.

\textbf{Visualization on Occluded Scenes.} To validate the robustness of our method in handling occluded scenes, we present additional visual results on both OCC3D-nuScenes and Openocc-nuScenes dataset. As shown in the first scene in Fig.~\ref{fig:vis_occlusion_failure}, our method is able to detect pedestrians that are partially occluded. As shown in the second scene, our approach performs well in identifying vehicles that are largely occluded by other vehicles. 

\textbf{Visualization on Low-light Scenes.} To validate the robustness of our method in handling low-light environments, we present additional visual results. As illustrated in the Fig.~\ref{fig:vis_night}, on the OCC3D-nuScenes, our model demonstrates the capability to recognize small objects, such as pedestrians and motorcycles, in low-light scenes, and it can effectively detect motorcycles at a considerable distance. 
\begin{figure*}[]
    \centering
    \includegraphics[width=0.95\linewidth]{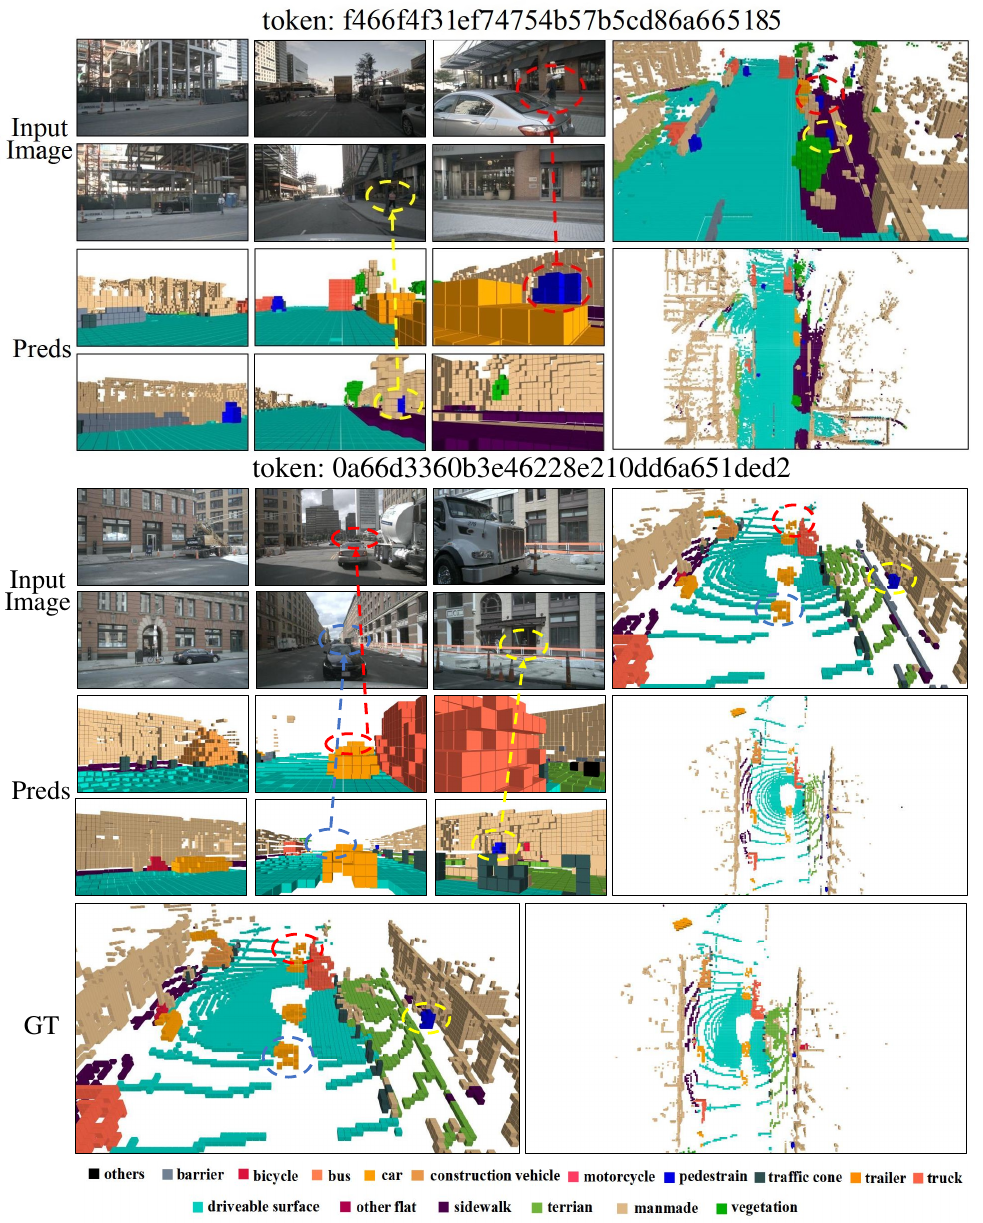}
    \caption{Visualizations for occlusion on OCC3D-nuScenes validation set. For each scene, the six images in the \textit{``Input Images''} line left are the inputs to our model captured by font-left, front, front-right, back-right, back, and back-right cameras. The six images in the \textit{``Preds''} line left denote our prediction results with the corresponding views as the inputs. The two images on the right provide a global view of our predictions. The two images in the \textit{``GT''} line provide a global view of ground truth.}
    \label{fig:vis_occlusion_failure}
\end{figure*}
\begin{figure*}[]
    \centering
    \includegraphics[width=0.95\linewidth]{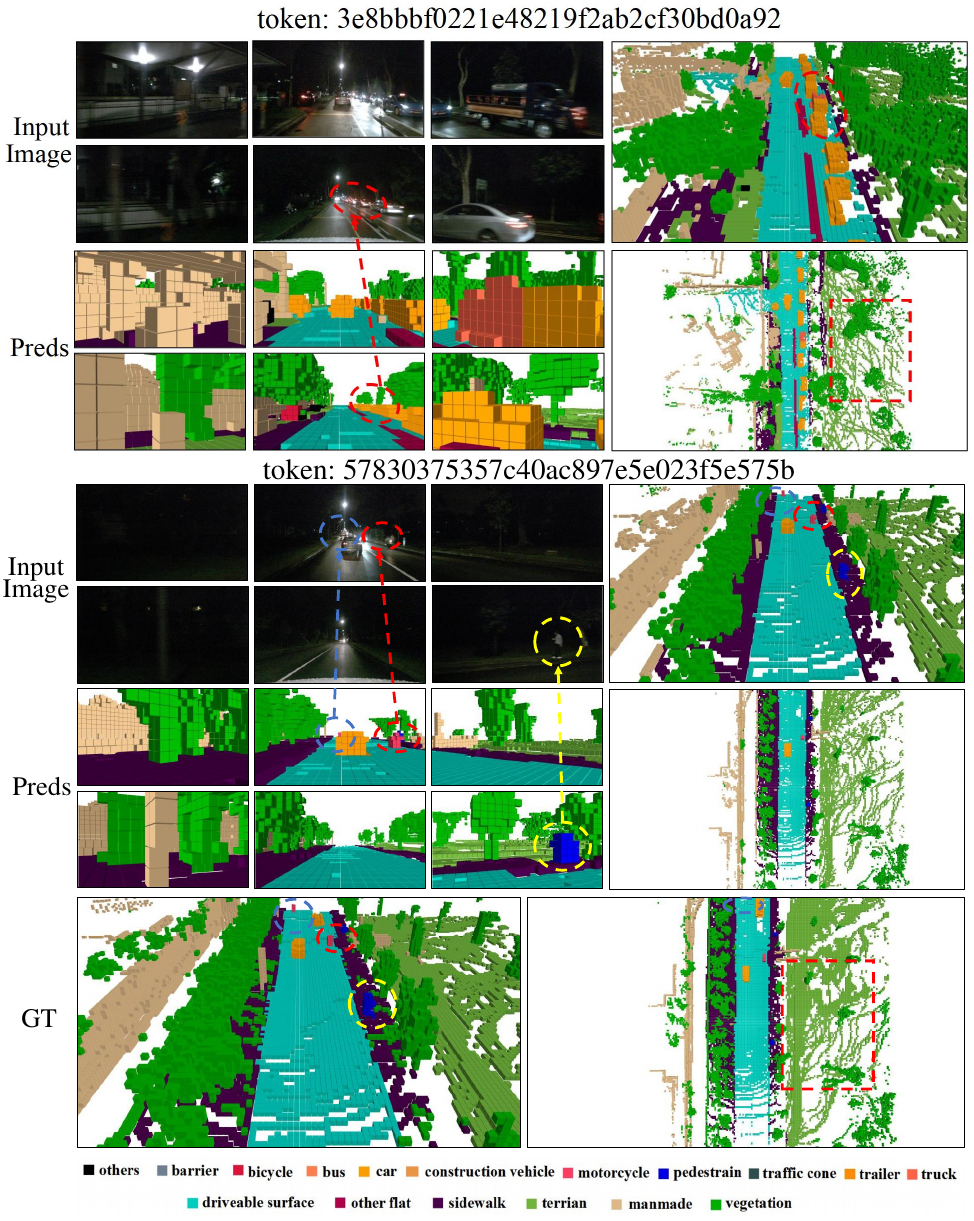}
    \caption{Visualizations for low-light environments on OCC3D-nuScenes validation set.}
    \label{fig:vis_night}
\end{figure*}

% \begin{figure*}[]
%     \centering
%     \includegraphics[width=0.95\linewidth]{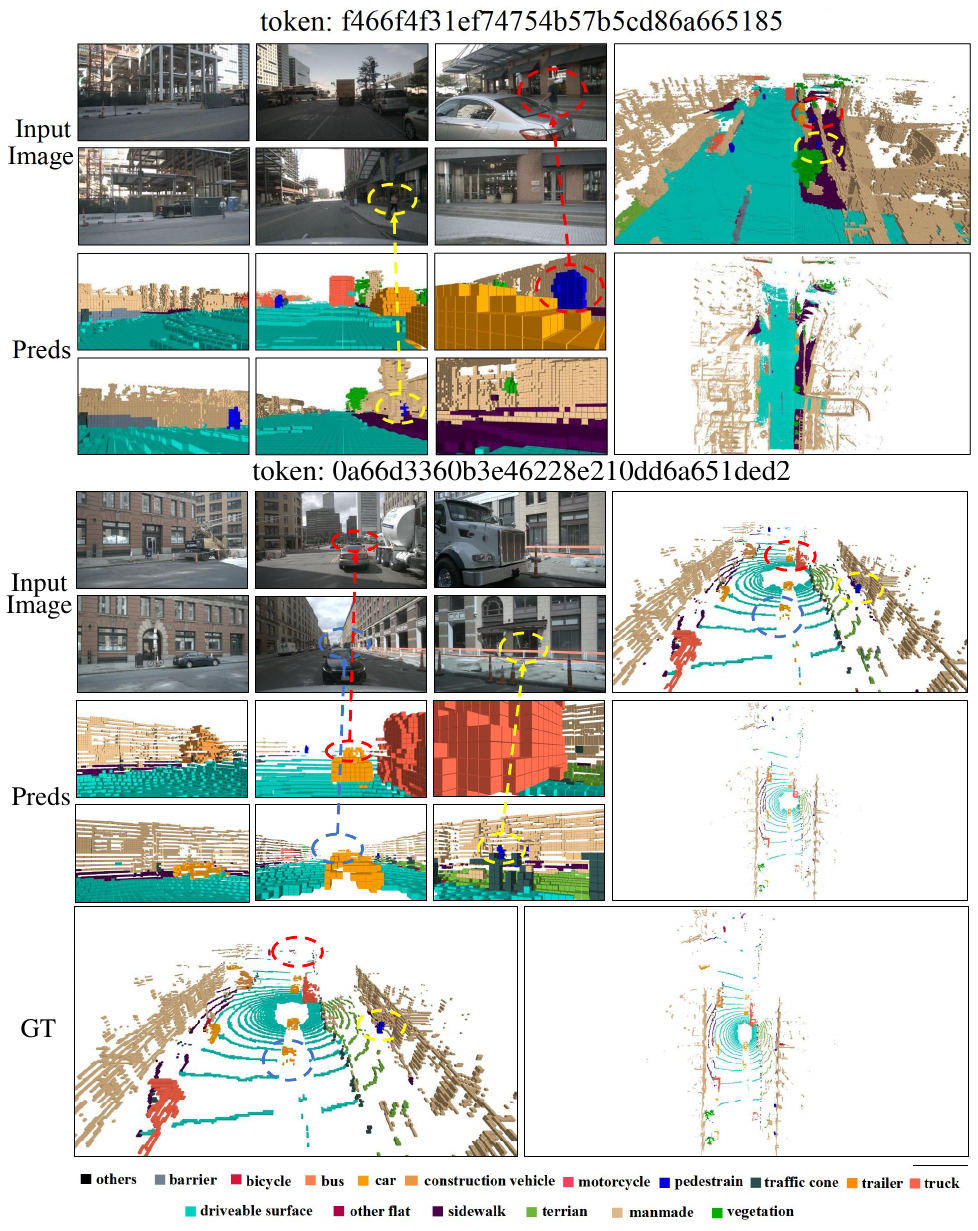}
%     \caption{Visualizations for occlusion on Openocc-nuScenes validation set. For each scene, the six images in the \textit{``Input Images''} line left are the inputs to our model captured by font-left, front, front-right, back-right, back, and back-right cameras. The six images in the \textit{``Preds''} line left denote our prediction results with the corresponding views as the inputs. The two images on the right provide a global view of our predictions. The two images in the \textit{``GT''} line provide a global view of ground truth.}
%     \label{fig:vis_occlusion_open}
% \end{figure*}
% \begin{figure*}[]
%     \centering
%     \includegraphics[width=\linewidth]{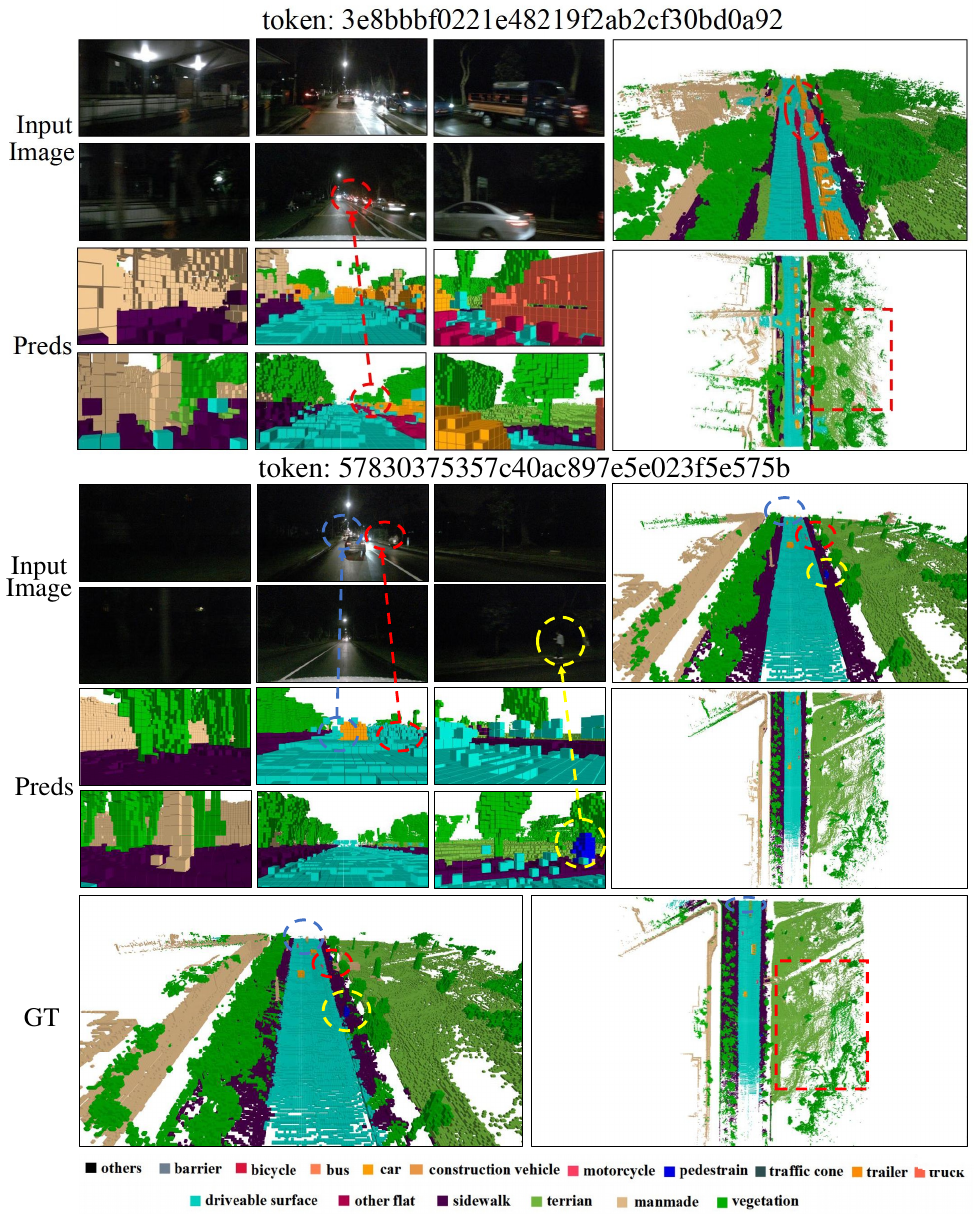}
%     \caption{Visualizations for low-light environments on Openocc-nuScenes validation set.}
%     \label{fig:vis_night_open}
% \end{figure*}
